# Supplementary material for: Nowcasting Gentrification Using Airbnb Data
Source: arXiv:2101.05924 source file (2021-01-18)
Supplement: Supplementary file 1 [file corr1_age.tex]

\begin{table}[ht]
    \mytablesize
    \tabcolsep 1pt
    \centering
    \caption{Linear Correlation ($r$) between Age and Airbnb Data.} 
	\begin{tabular}{p{5cm} rl @{\hskip 10pt} rl @{\hskip 10pt} rl}
        \toprule
        Airbnb Data Variables & 
        \multicolumn{2}{c}{New York} & 
        \multicolumn{2}{c}{Los Angeles} & 
        \multicolumn{2}{c}{London}\\ 
        \midrule
        \textit{Structured Data Features} \\
        \hspace{1em} \#~Listings            & *** & \Posbar{0.420} &  & \Posbar{0.077} &  & \Negbar{-0.011} \\
        \hspace{1em} \#~Reviews             & *** & \Posbar{0.430} & & \Posbar{0.067} & & \Negbar{-0.023} \\
        \hspace{1em} Price                  &  & \Posbar{0.023} & * & \Negbar{-0.245} &  & \Negbar{-0.007} \\
        \hspace{1em} \#~Bedrooms            &  *   & \Negbar{-0.188} & & \Posbar{0.203}&  & \Negbar{-0.109} \\
        \hspace{1em} Star-Rating            &     & \Negbar{-0.135} &     & \Negbar{-0.173}&     & \Negbar{-0.038} \\
        \hspace{1em} Location Star-Rating   & **  & \Negbar{-0.254} &     & \Negbar{-0.174} & & \Negbar{-0.045}\\
        \midrule
        \textit{Unstructured Data Features} \\
        \hspace{1em} Review Length                              &  & \Posbar{0.184} & *  & \Negbar{-0.227} &  & \Negbar{-0.026} \\
        \hspace{1em} Location Words                             &  & \Posbar{0.053} &  & \Negbar{-0.074} & & \Posbar{0.008} \\
        \hspace{1em} Sentiment                                  &  & \Posbar{0.057} &     & \Negbar{-0.036} & * & \Negbar{-0.132} \\
        \hspace{1em} Sentiment in Location Reviews              &  & \Posbar{0.083} &  & \Negbar{-0.143} & ** & \Negbar{-0.159} \\
        \hspace{1em} LDA Component (Check-In)                   &     & \Posbar{0.051}&     & \Posbar{0.048}&  & \Posbar{0.091} \\
        \hspace{1em} LDA Component (Listing Characteristics)    &  & \Posbar{0.044}&     & \Posbar{0.018}&  **   & \Posbar{0.161} \\
        \hspace{1em} LDA Component (Location)                   &  & \Posbar{0.028} &  & \Posbar{0.010} & * & \Negbar{-0.143} \\
        \hspace{1em} LDA Component (Stay/Host)                  & ** & \Negbar{-0.238}&   & \Negbar{-0.144}& * & \Negbar{-0.106} \\
        \hspace{1em} LDA Component (Public Transportation)      &     & \Posbar{0.145} &     & N/A            &     & \Posbar{0.143} \\
        \hspace{1em} Doc2Vec Component (1)                      & *** & \Negbar{-0.344}& ** & \Posbar{0.313} & *** & \Negbar{-0.179} \\
        \midrule
        Disadvantaged Neighborhoods & \multicolumn{2}{c}{79} & \multicolumn{2}{c}{58} & \multicolumn{2}{c}{186} \\
        \bottomrule
         \multicolumn{7}{l}{\textit{Note: Change in Age between 1998-2002 and 2013-2017; Significance levels: }{$^{*}$p$<$0.1; $^{**}$p$<$0.05; $^{***}$p$<$0.01}} \\
	\end{tabular}
    \label{table:corr_age}
\end{table}
