# Supplementary material for: Nowcasting Gentrification Using Airbnb Data
Source: arXiv:2101.05924 source file (2021-01-18)
Supplement: Supplementary file 2 [file corr2_edu.tex]

\begin{table}[ht]
    \mytablesize
    \tabcolsep 1pt
    \centering
    \caption{Linear Correlation ($r$) between Education and Airbnb Data.} 
	\begin{tabular}{p{5cm} rl @{\hskip 10pt} rl @{\hskip 10pt} rl}
        \toprule
        Airbnb Data Variables & 
        \multicolumn{2}{c}{New York} & 
        \multicolumn{2}{c}{Los Angeles} & 
        \multicolumn{2}{c}{London}\\ 
        \midrule
        \textit{Structured Data Features} \\
        \hspace{1em} \#~Listings            & *** & \Posbar{0.716} & *** & \Posbar{0.375} & *** & \Posbar{0.349} \\
        \hspace{1em} \#~Reviews             & *** & \Posbar{0.694} & *** & \Posbar{0.362} & *** & \Posbar{0.264} \\
        \hspace{1em} Price                  & *** & \Posbar{0.525} & ** & \Posbar{0.324} & *** & \Posbar{0.215} \\
        \hspace{1em} \#~Bedrooms            &     & \Posbar{0.108} & ***  & \Negbar{-0.357}& ***  & \Posbar{0.209} \\
        \hspace{1em} Star-Rating            &     & \Posbar{0.051} &     & \Negbar{-0.122}& *    & \Posbar{0.122} \\
        \hspace{1em} Location Star-Rating   & **  & \Posbar{0.230} &  **   & \Posbar{0.294} & *** & \Posbar{0.194}\\
        \midrule
        \textit{Unstructured Data Features} \\
        \hspace{1em} Review Length                              & *** & \Posbar{0.602} & **  & \Posbar{0.334} & *** & \Posbar{0.351} \\
        \hspace{1em} Location Words                             & *** & \Posbar{0.530} & *** & \Posbar{0.525} & *** & \Posbar{0.214} \\
        \hspace{1em} Sentiment                                  & *** & \Posbar{0.455} &     & \Posbar{0.162} & *** & \Posbar{0.259} \\
        \hspace{1em} Sentiment in Location Reviews              & *** & \Posbar{0.557} & **   & \Posbar{0.297} & *** & \Posbar{0.297} \\
        \hspace{1em} LDA Component (Check-In)                   &     & \Posbar{0.033}&     & \Negbar{-0.120}& ***  & \Negbar{-0.207} \\
        \hspace{1em} LDA Component (Listing Characteristics)    & *** & \Negbar{-0.437}&     & \Negbar{-0.202}&     & \Negbar{-0.062} \\
        \hspace{1em} LDA Component (Location)                   & *** & \Posbar{0.487} & *** & \Posbar{0.508} & *** & \Posbar{0.321} \\
        \hspace{1em} LDA Component (Stay/Host)                  & *** & \Negbar{-0.339}& **  & \Negbar{-0.330}&  & \Negbar{-0.103} \\
        \hspace{1em} LDA Component (Public Transportation)      &     & \Posbar{0.017} &     & N/A            &     & \Posbar{0.044} \\
        \hspace{1em} Doc2Vec Component (1)                      & *** & \Negbar{-0.683}& *** & \Posbar{0.566} & *** & \Negbar{-0.329} \\
        \midrule
        Disadvantaged Neighborhoods & \multicolumn{2}{c}{79} & \multicolumn{2}{c}{58} & \multicolumn{2}{c}{186} \\
        \bottomrule
         \multicolumn{7}{l}{\textit{Note: Change in Education between 1998-2002 and 2013-2017; Significance levels: }{$^{*}$p$<$0.1; $^{**}$p$<$0.05; $^{***}$p$<$0.01}} \\
	\end{tabular}
    \label{table:corr_edu}
\end{table}
