# Supplementary material for: Nowcasting Gentrification Using Airbnb Data
Source: arXiv:2101.05924 source file (2021-01-18)
Supplement: Supplementary file 3 [file corr3_income.tex]

\begin{table}[ht]
    \mytablesize
    \tabcolsep 1pt
    \centering
    \caption{Linear Correlation ($r$) between Income and Airbnb Data.} 
	\begin{tabular}{p{5cm} rl @{\hskip 10pt} rl @{\hskip 10pt} rl}
        \toprule
        Airbnb Data Variables & 
        \multicolumn{2}{c}{New York} & 
        \multicolumn{2}{c}{Los Angeles} & 
        \multicolumn{2}{c}{London}\\ 
        \midrule
        \textit{Structured Data Features} \\
        \hspace{1em} \#~Listings            & *** & \Posbar{0.564} & ** & \Posbar{0.330} & *** & \Posbar{0.312} \\
        \hspace{1em} \#~Reviews             & *** & \Posbar{0.521} & ** & \Posbar{0.310} & *** & \Posbar{0.300} \\
        \hspace{1em} Price                  & *** & \Posbar{0.479} & ** & \Posbar{0.311} & *** & \Posbar{0.230} \\
        \hspace{1em} \#~Bedrooms            &     & \Posbar{0.108} & **  & \Negbar{-0.318}&   & \Posbar{0.077} \\
        \hspace{1em} Star-Rating            &     & \Posbar{0.106} &     & \Negbar{-0.120}&     & \Posbar{0.064} \\
        \hspace{1em} Location Star-Rating   & ***  & \Posbar{0.415} &  *   & \Posbar{0.237} & * & \Posbar{0.139}\\
        \midrule
        \textit{Unstructured Data Features} \\
        \hspace{1em} Review Length                              & *** & \Posbar{0.367} & ***  & \Posbar{0.336} & *** & \Posbar{0.286} \\
        \hspace{1em} Location Words                             & *** & \Posbar{0.444} & *** & \Posbar{0.426} & *** & \Posbar{0.293} \\
        \hspace{1em} Sentiment                                  & *** & \Posbar{0.318} &     & \Posbar{0.200} & & \Posbar{0.096} \\
        \hspace{1em} Sentiment in Location Reviews              & *** & \Posbar{0.345} & ***   & \Posbar{0.336} & * & \Posbar{0.142} \\
        \hspace{1em} LDA Component (Check-In)                   &     & \Negbar{-0.045}&     & \Negbar{-0.125}&  & \Negbar{-0.077} \\
        \hspace{1em} LDA Component (Listing Characteristics)    & *** & \Negbar{-0.380}&   *  & \Negbar{-0.231}&     & \Posbar{0.086} \\
        \hspace{1em} LDA Component (Location)                   & *** & \Posbar{0.459} & *** & \Posbar{0.425} & *** & \Posbar{0.216} \\
        \hspace{1em} LDA Component (Stay/Host)                  & * & \Negbar{-0.216}& *  & \Negbar{-0.247}& *** & \Negbar{-0.207} \\
        \hspace{1em} LDA Component (Public Transportation)      &     & \Negbar{-0.078} &     & N/A            &     & \Posbar{0.104} \\
        \hspace{1em} Doc2Vec Component (1)                      & *** & \Negbar{-0.653}& *** & \Posbar{0.447} & *** & \Negbar{-0.383} \\
        \midrule
        Disadvantaged Neighborhoods & \multicolumn{2}{c}{79} & \multicolumn{2}{c}{58} & \multicolumn{2}{c}{186} \\
        \bottomrule
         \multicolumn{7}{l}{\textit{Note: Change in Income between 1998-2002 and 2013-2017; Significance levels: }{$^{*}$p$<$0.1; $^{**}$p$<$0.05; $^{***}$p$<$0.01}} \\
	\end{tabular}
    \label{table:corr_income}
\end{table}
