# Supplementary material for: Nowcasting Gentrification Using Airbnb Data
Source: arXiv:2101.05924 source file (2021-01-18)
Supplement: Supplementary file 4 [file corr4_rent.tex]

\begin{table}[ht]
    \mytablesize
    \tabcolsep 1pt
    \centering
    \caption{Linear Correlation ($r$) between Rent and Airbnb Data.} 
	\begin{tabular}{p{5cm} rl @{\hskip 10pt} rl @{\hskip 10pt} rl}
        \toprule
        Airbnb Data Variables & 
        \multicolumn{2}{c}{New York} & 
        \multicolumn{2}{c}{Los Angeles} & 
        \multicolumn{2}{c}{London}\\ 
        \midrule
        \textit{Structured Data Features} \\
        \hspace{1em} \#~Listings            & *** & \Posbar{0.595} &  & \Posbar{0.202} & *** & \Posbar{0.534} \\
        \hspace{1em} \#~Reviews             & *** & \Posbar{0.530} &  & \Posbar{0.184} & *** & \Posbar{0.473} \\
        \hspace{1em} Price                  & *** & \Posbar{0.379} & ** & \Posbar{0.286} & *** & \Posbar{0.355} \\
        \hspace{1em} \#~Bedrooms            &     & \Posbar{0.075} & **  & \Negbar{-0.280}& *  & \Posbar{0.136} \\
        \hspace{1em} Star-Rating            &     & \Posbar{0.045} &  *   & \Negbar{-0.240}&     & \Posbar{0.046} \\
        \hspace{1em} Location Star-Rating   & ***  & \Posbar{0.335} &     & \Posbar{0.182} & *** & \Posbar{0.351}\\
        \midrule
        \textit{Unstructured Data Features} \\
        \hspace{1em} Review Length                              & *** & \Posbar{0.419} & *  & \Posbar{0.241} & *** & \Posbar{0.224} \\
        \hspace{1em} Location Words                             & ** & \Posbar{0.266} & ** & \Posbar{0.315} & *** & \Posbar{0.468} \\
        \hspace{1em} Sentiment                                  & *** & \Posbar{0.306} &     & \Posbar{0.024} & *** & \Posbar{0.211} \\
        \hspace{1em} Sentiment in Location Reviews              & *** & \Posbar{0.345} &    & \Posbar{0.170} & ** & \Posbar{0.182} \\
        \hspace{1em} LDA Component (Check-In)                   &     & \Negbar{-0.123}&     & \Posbar{0.108}& **  & \Negbar{-0.185} \\
        \hspace{1em} LDA Component (Listing Characteristics)    & ** & \Negbar{-0.222}&     & \Negbar{-0.143}&     & \Posbar{0.085} \\
        \hspace{1em} LDA Component (Location)                   & *** & \Posbar{0.442} & *** & \Posbar{0.336} & *** & \Posbar{0.456} \\
        \hspace{1em} LDA Component (Stay/Host)                  & ** & \Negbar{-0.239}& **  & \Negbar{-0.273}& *** & \Negbar{-0.269} \\
        \hspace{1em} LDA Component (Public Transportation)      &     & \Negbar{-0.117} &     & N/A            &     & \Negbar{-0.014} \\
        \hspace{1em} Doc2Vec Component (1)                      & *** & \Negbar{-0.578}& *** & \Posbar{0.507} & *** & \Negbar{-0.312} \\
        \midrule
        Disadvantaged Neighborhoods & \multicolumn{2}{c}{79} & \multicolumn{2}{c}{58} & \multicolumn{2}{c}{186} \\
        \bottomrule
         \multicolumn{7}{l}{\textit{Note: Change in Rent between 1998-2002 and 2013-2017; Significance levels: }{$^{*}$p$<$0.1; $^{**}$p$<$0.05; $^{***}$p$<$0.01}} \\
	\end{tabular}
    \label{table:corr_rent}
\end{table}
