# Supplementary material for: Nowcasting Gentrification Using Airbnb Data
Source: arXiv:2101.05924 source file (2021-01-18)
Supplement: Supplementary file 5 [file corr5_race.tex]

\begin{table}[ht]
    \mytablesize
    \tabcolsep 1pt
    \centering
    \caption{Linear Correlation ($r$) between Race and Airbnb Data.} 
	\begin{tabular}{p{5cm} rl @{\hskip 10pt} rl @{\hskip 10pt} rl}
        \toprule
        Airbnb Data Variables & 
        \multicolumn{2}{c}{New York} & 
        \multicolumn{2}{c}{Los Angeles} & 
        \multicolumn{2}{c}{London}\\ 
        \midrule
        \textit{Structured Data Features} \\
        \hspace{1em} \#~Listings            & *** & \Posbar{0.675} & *** & \Posbar{0.466} && N/A \\
        \hspace{1em} \#~Reviews             & *** & \Posbar{0.668} & *** & \Posbar{0.450} && N/A \\
        \hspace{1em} Price                  & *** & \Posbar{0.427} & *** & \Posbar{0.572} && N/A \\
        \hspace{1em} \#~Bedrooms            &     & \Posbar{0.003} & **  & \Negbar{-0.300} && N/A \\
        \hspace{1em} Star-Rating            &     & \Negbar{-0.050} &     & \Negbar{-0.022} && N/A \\
        \hspace{1em} Location Star-Rating   &   & \Posbar{0.078} &  ***   & \Posbar{0.404} && N/A \\
        \midrule
        \textit{Unstructured Data Features} \\
        \hspace{1em} Review Length                              & *** & \Posbar{0.512} & ***  & \Posbar{0.417} && N/A \\
        \hspace{1em} Location Words                             & *** & \Posbar{0.365} & *** & \Posbar{0.459} && N/A \\
        \hspace{1em} Sentiment                                  & *** & \Posbar{0.347} &  **   & \Posbar{0.319} && N/A \\
        \hspace{1em} Sentiment in Location Reviews              & *** & \Posbar{0.442} & ***   & \Posbar{0.376} && N/A \\
        \hspace{1em} LDA Component (Check-In)                   &     & \Posbar{0.015}&     & \Negbar{-0.172} && N/A \\
        \hspace{1em} LDA Component (Listing Characteristics)    & ** & \Negbar{-0.277}&  ***   & \Negbar{-0.338} && N/A \\
        \hspace{1em} LDA Component (Location)                   & *** & \Posbar{0.481} & *** & \Posbar{0.495} && N/A \\
        \hspace{1em} LDA Component (Stay/Host)                  & *** & \Negbar{-0.352}&\textbf{}  & \Negbar{-0.215} && N/A \\
        \hspace{1em} LDA Component (Public Transportation)      &     & \Negbar{-0.070} &     & N/A            && N/A \\
        \hspace{1em} Doc2Vec Component (1)                      & *** & \Negbar{-0.665}& *** & \Posbar{0.443} && N/A \\
        \midrule
        Disadvantaged Neighborhoods & \multicolumn{2}{c}{79} & \multicolumn{2}{c}{58} & \multicolumn{2}{c}{186} \\
        \bottomrule
         \multicolumn{7}{l}{\textit{Note: Change in Race between 1998-2002 and 2013-2017; Significance levels: }{$^{*}$p$<$0.1; $^{**}$p$<$0.05; $^{***}$p$<$0.01}} \\
	\end{tabular}
    \label{table:corr_rent}
\end{table}
